# Supplementary material for: DeepTAM: Deep Tracking and Mapping
Source: arXiv:1808.01900 source file (2018-08-07)
Supplement: Supplementary file 1 [file deeptam_supplement.pdf]

# DeepTAM: Deep Tracking and Mapping
# Supplementary Material

## 1 Tracking Network Implementation Details

Fig. 1 shows the operations and parameters of the ConvNet parts for the three tracking networks.

### 1.1 Rendering

The input to the ConvNets is the current camera image and the rendered virtual keyframe. To pass as much information as possible to the ConvNet, we render two image and depth map pairs. We use the depth tests GREATER and LESS to render the images and depth maps. The depth test GREATER generates an image and an inverse depth map pair which corrsponds to what can actually be seen from the specified viewpoint. The depth test LESS generates an image and depth map which shows the occluded parts (we assume that there are at most two depth layers). We use simple point-based rendering to generate images and depth maps.

## 2 Mapping Network Implementation

Fig. 3 shows the operations and parameters of the ConvNets of the mapping module.

## 3 Runtimes

Tab. 1 shows the runtimes of each network component of our approach. The tracking can run in real-time. For the mapping we use the cost volume to collect information from incoming frames. We do not run the fixed band and narrow band modules at frame rate, but invoke them once enough frames have been collected.

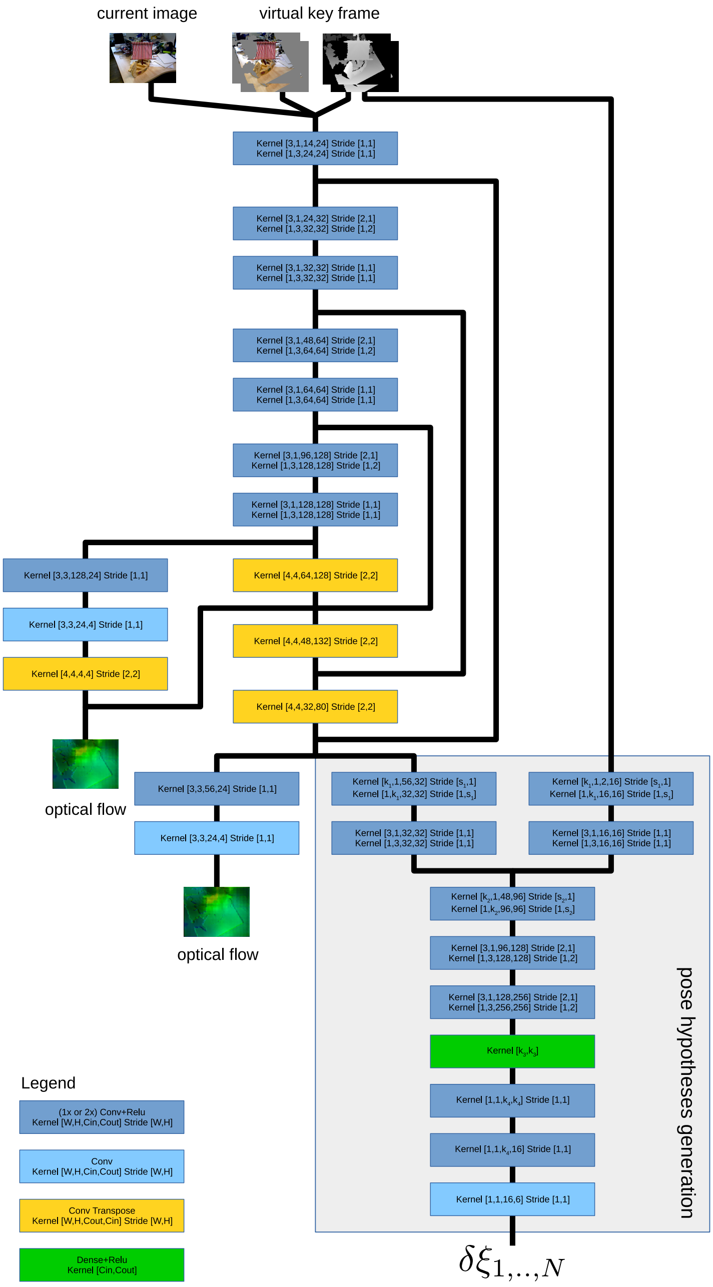


**Fig. 1.** Tracking network parameters. The shared encoder decoder configuration is identical for all resolution levels. The pose hypotheses generation part uses slightly different kernel size and stride parameters for each resolution level. The changing parameters for the resolution levels $[60 \times 80, 120 \times 160, 240 \times 320]$ are: $k_1 : [3, 5, 5]$, $s_1 : [2, 4, 4]$, $k_2 : [3, 3, 5]$, $s_2 : [2, 2, 4]$, $k_3 : [1536, 1536, 2048]$, $k_4 : [24, 24, 32]$.

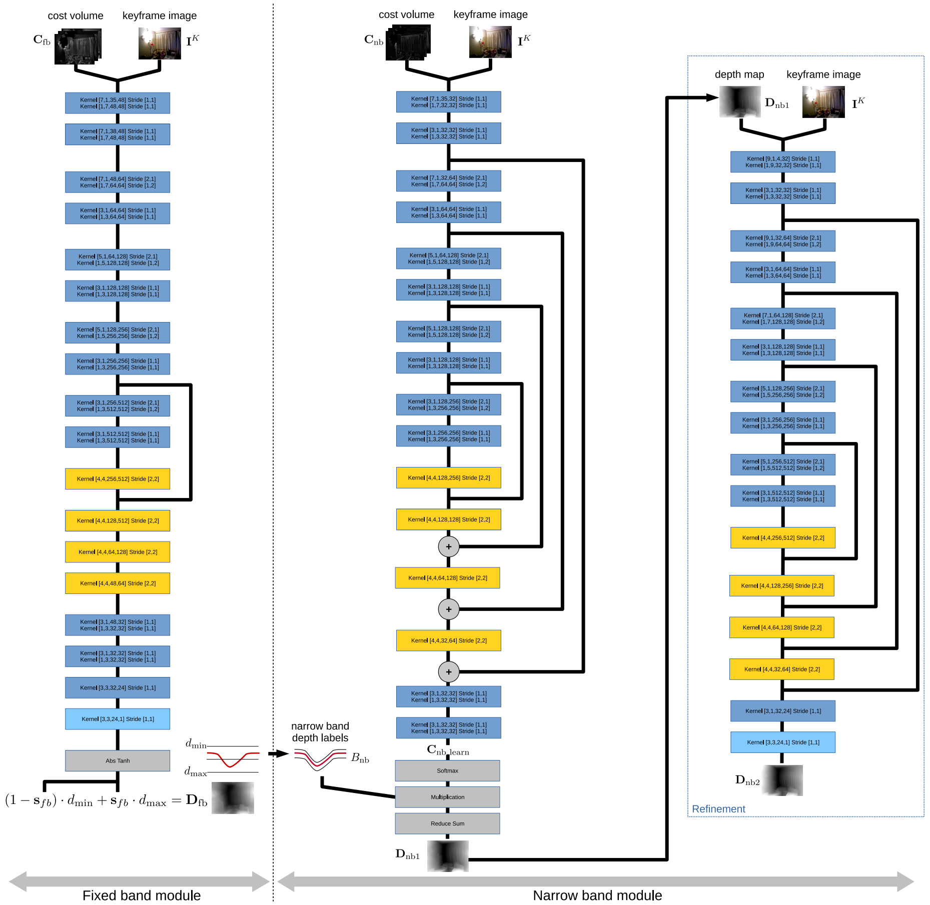


**Fig. 2.** Mapping networks parameters. The mapping consists of two modules: fixed band module and narrow band module. **Fixed band module**: This module takes the keyframe image $\mathbf{I}^K$ $(320 \times 240 \times 3)$ and the cost volume $\mathbf{C}_{fb}$ $(320 \times 240 \times 32)$ generated with 32 depth labels equally spaced in the range [0.01, 2.5] as inputs and outputs an interpolation factor $s_{fb}$ $(320 \times 240 \times 1)$. The fixed band depth estimation is computed as $\mathbf{D}_{fb} = (1 - \mathbf{s}_{fb}) \cdot d_{min} + \mathbf{s}_{fb} \cdot d_{max}$. **Narrow band module**: The narrow band module is run iteratively; in each iteration we build a cost volume $\mathbf{C}_{nb}$ from a set of depth labels distributed around the current depth estimation with a band width $\sigma_{nb}$ of 0.0125. It consists of two encoder-decoder pairs. The first pair gets the cost volume $\mathbf{C}_{nb}$ $(320 \times 240 \times 32)$ and the keyframe image $\mathbf{I}^K$ $(320 \times 240 \times 3)$ as inputs and generates a learned cost volume $\mathbf{C}_{nb\_learn}$ $(320 \times 240 \times 32)$. The depth map is then obtained using a differentiable soft argmin operation [3]: $\mathbf{D}_{nb1} = \sum_{d \in \mathbf{B}_{nb}} \mathbf{B}_{nb} \times \mathrm{softmax}(-\mathbf{C}_{nb\_learn})$. The second encoder-decoder pair gets the current depth estimation $\mathbf{D}_{nb1}$ and the keyframe image $\mathbf{I}^K$ and produces a refined depth $\mathbf{D}_{nb2}$.

| | Tracking | Cost volume | Fixed band | Narrow band |
|---|---|---|---|---|
| Mean | 0.0227 | 0.0164 | 0.0181 | 0.0359 |
| Min | 0.0203 | 0.0153 | 0.0171 | 0.0347 |
| Max | 0.0251 | 0.0168 | 0.0190 | 0.0393 |

**Table 1.** Runtime in seconds for each component of our system. The statistic is computed excluding outliers. The **Tracking** time is the time required for a forward pass through all three resolution levels including render time for the virtual keyframe. The isolated tracking component runs with about 44 Hz. The runtimes for **Cost volume** describe the time to compute and add the matching costs of a new frame. The cost volume generation is implemented with Tensorflow ops and has some overhead. The **Narrow band** time is the time per iteration. All runtimes have been measured on an NVIDIA GTX 1070.

# 4 Results

Tab. 2 shows an extended evaluation on the TUM RGB-D benchmark for the freiburg1 sequences with public ground truth and the validation sets with secret ground truth.
Fig. 3 shows more examples of our mapping component in comparison with SGM [2], DTAM [5] and DeMoN [8].

# 5 Generalization

It is well known that learning-based methods easily overfit. To prevent this problem we trained and tested on diverse datasets, which covers indoor and outdoor scenarios and consists of realistic and artificial data. Additionally, we carefully design our network architecture to avoid overfitting. Tab. 2 shows our results on the TUM RGB-D benchmark, which was not part of our training data. In addition, Fig. 4 demonstrates that our mapping module also generalizes well to KITTI datasets without any finetuning.

| | Tracking | | | | Tracking and mapping | |
|---|---|---|---|---|---|---|
| Sequence | RGB-D SLAM Kerl *et al.* [4] | Ours (w/o flow) | Ours (single pose) | Ours | CNN-SLAM* Tateno *et al.* [7] | Ours |
| fr1/360 | 0.119 | 0.079 | 0.070 | **0.063** | 0.839 | **0.133** |
| fr1/360 (v) | 0.125 | 0.069 | 0.065 | **0.054** | 0.500 | **0.116** |
| fr1/desk | **0.030** | 0.051 | 0.048 | 0.033 | 0.175 | **0.130** |
| fr1/desk (v) | 0.037 | 0.042 | 0.031 | **0.027** | 0.095 | **0.078** |
| fr1/desk2 | 0.055 | 0.064 | 0.054 | **0.046** | 0.236 | **0.124** |
| fr1/desk2 (v) | 0.020 | 0.025 | 0.020 | **0.017** | 0.115 | **0.055** |
| fr1/floor | 0.090 | 0.095 | 0.091 | **0.081** | **0.282** | **0.282** |
| fr1/plant | 0.036 | 0.038 | 0.028 | **0.027** | **0.178** | 0.299 |
| fr1/plant (v) | 0.062 | 0.063 | 0.060 | **0.057** | **0.150** | 0.165 |
| fr1/room | 0.048 | 0.059 | 0.048 | **0.040** | 0.169 | **0.138** |
| fr1/room (v) | 0.042 | 0.051 | 0.041 | **0.039** | 0.445 | **0.084** |
| fr1/rpy | **0.043** | 0.052 | 0.045 | 0.046 | 0.074 | **0.046** |
| fr1/rpy (v) | 0.082 | 0.070 | **0.063** | 0.065 | 0.261 | **0.052** |
| fr1/teddy | 0.067 | 0.067 | **0.058** | 0.059 | 0.207 | **0.164** |
| fr1/xzy | 0.024 | 0.029 | 0.021 | **0.017** | 0.060 | **0.045** |
| fr1/xzy (v) | 0.051 | 0.030 | 0.021 | **0.019** | 0.206 | **0.054** |
| average | 0.058 | 0.055 | 0.047 | **0.043** | 0.250 | **0.123** |

**Table 2.** Evaluation of our tracking (left part) and the combined mapping and tracking (right part) on the RGB-D benchmark [6]. The values describe the translational RMSE in $[m/s]$. The validation sets are marked with (v). **Tracking:** We compare the performance of our tracking network against the RGB-D SLAM method of Kerl *et al.* [4]. Numbers for Kerl *et al.* [4] correspond to the frame-to-keyframe odometry evaluation and have been copied from their paper. Note that Kerl *et al.* [4] uses the camera image *and* the depth stream for computing the poses, while our approach uses the depth stream only for keyframes and is limited to photometric alignment. **Ours (single pose)** is our tracking with generating just a single pose hypothesis and deactivated $\mathcal{L}_{\text{uncertainty}}$. **Ours** is our tracking network with 64 pose hypotheses and the mean as final estimate. Both versions use the depth stream to obtain the depth for keyframes. **Tracking and mapping:** We compare our tracking and mapping against CNN-SLAM by Tateno *et al.* [7]. * For a fair comparison CNN-SLAM is run without pose graph optimization. To avoid a bias in the initialization **Ours** uses the depth prediction from CNN-SLAM for the first frame of each sequence and then switches to our combined tracking and mapping.

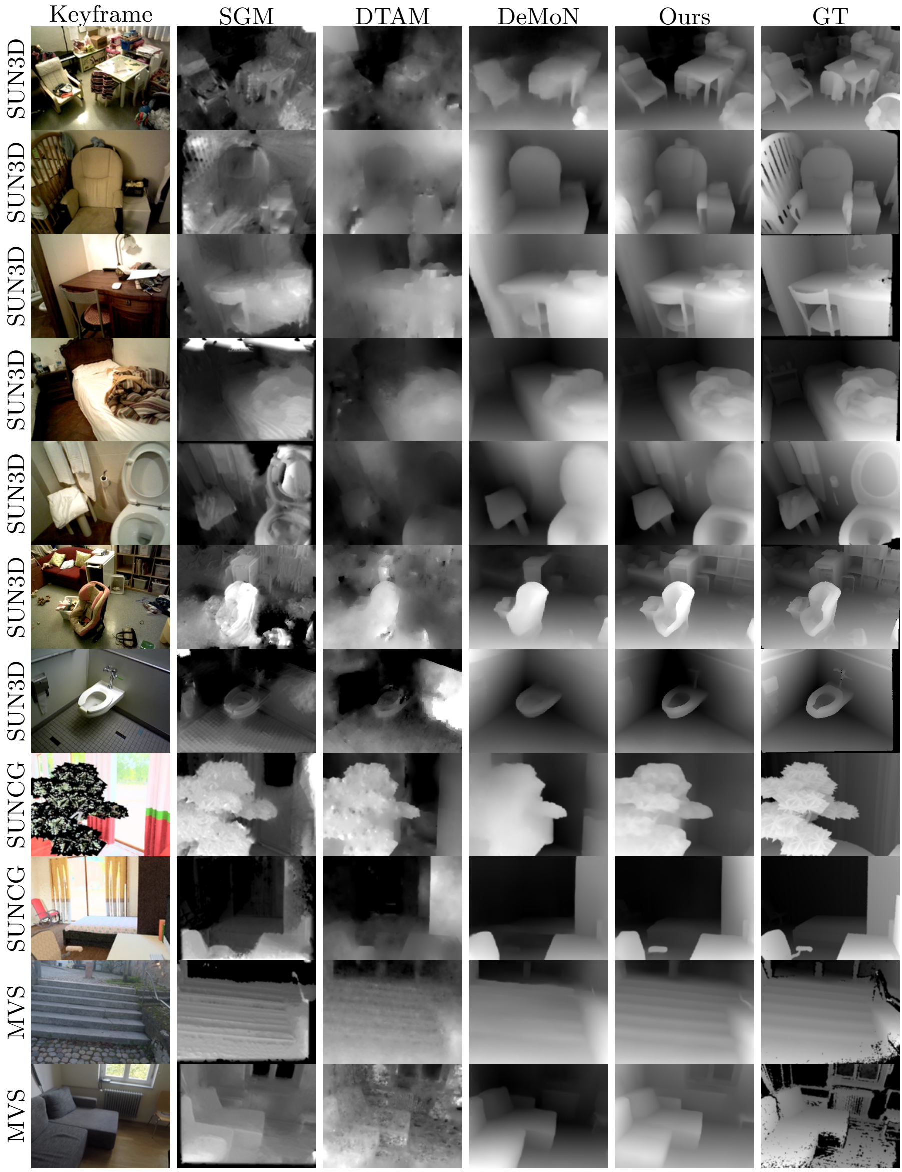


**Fig. 3.** Qualitative depth prediction comparison for sequences with 10 frames. DeMoN uses only the first and last frame of each sequence.

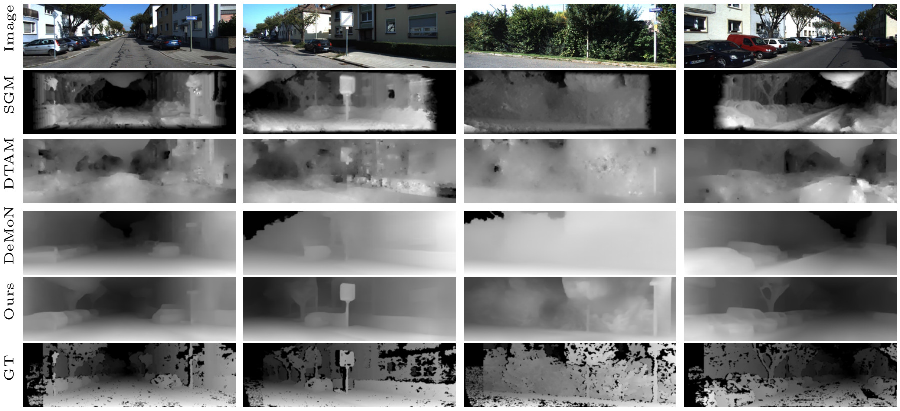


**Fig. 4.** Generalization experiment on KITTI [1]. SGM, DTAM and Ours use a sequence of 5 frames from the left color camera, while for DeMoN we only use the first and last frame of each sequence. We show pseudo GT as a reference, which was obtained by computing the disparity of the corresponding rectified and synchronized stereo pairs. KITTI is an urban scene dataset captured with a wide-angle camera, which differs from our training data significantly. Further, due to the dominant forward motion pattern of the dataset the epipole is within the visible image borders, which makes depth estimation especially difficult. Without finetuning our method generalizes well to this dataset.

## References

1. Geiger, A., Lenz, P., Urtasun, R.: Are we ready for autonomous driving? the kitti vision benchmark suite. In: Computer Vision and Pattern Recognition (CVPR), 2012 IEEE Conference On. pp. 3354–3361. IEEE (2012)
2. Hirschmüller, H.: Accurate and efficient stereo processing by semi-global matching and mutual information. In: 2005 IEEE Computer Society Conference on Computer Vision and Pattern Recognition (CVPR'05). vol. 2, pp. 807–814 vol. 2 (Jun 2005). https://doi.org/10.1109/CVPR.2005.56
3. Kendall, A., Martirosyan, H., Dasgupta, S., Henry, P.: End-to-End Learning of Geometry and Context for Deep Stereo Regression. In: 2017 IEEE International Conference on Computer Vision (ICCV). pp. 66–75 (Oct 2017). https://doi.org/10.1109/ICCV.2017.17
4. Kerl, C., Sturm, J., Cremers, D.: Dense visual SLAM for RGB-D cameras. In: 2013 IEEE/RSJ International Conference on Intelligent Robots and Systems. pp. 2100–2106 (Nov 2013). https://doi.org/10.1109/IROS.2013.6696650
5. Newcombe, R.A., Lovegrove, S., Davison, A.: DTAM: Dense tracking and mapping in real-time. In: 2011 IEEE International Conference on Computer Vision (ICCV). pp. 2320–2327 (2011). https://doi.org/10.1109/ICCV.2011.6126513
6. Sturm, J., Engelhard, N., Endres, F., Burgard, W., Cremers, D.: A benchmark for the evaluation of RGB-D SLAM systems. In: 2012 IEEE/RSJ International Conference on Intelligent Robots and Systems. pp. 573–580 (Oct 2012). https://doi.org/10.1109/IROS.2012.6385773
7. Tateno, K., Tombari, F., Laina, I., Navab, N.: CNN-SLAM: Real-Time Dense Monocular SLAM with Learned Depth Prediction. In: 2017 IEEE Conference on Computer Vision and Pattern Recognition (CVPR). pp. 6565–6574 (Jul 2017). https://doi.org/10.1109/CVPR.2017.695
8. Ummenhofer, B., Zhou, H., Uhrig, J., Mayer, N., Ilg, E., Dosovitskiy, A., Brox, T.: DeMoN: Depth and Motion Network for Learning Monocular Stereo. In: IEEE Conference on Computer Vision and Pattern Recognition (CVPR) (2017)
